# Supplementary material for: Interpreting Interpretations: Organizing Attribution Methods by Criteria
Source: arXiv:2002.07985 source file (2020-04-04)
Supplement: Supplementary file 1 [file 07-Appendix.tex]

\begin{proposition}
If an attribution method $A$ satisfy both sensitivity-$(N-n_1)$ and sensitivity-$(N-n_2)$, where $N$ is the total number of pixels, then $$S^k_p(X, A) = 0$$ under the condition  \label{pro:2}
\begin{equation}
    \sum^{n_1}_i s_i = \sum^{n_2}_j s_j = k S(A, X)
\end{equation}
\begin{equation}
    s_i \in \pi^+_A(X), s_j \in \hat{\pi}^+_A(X), k\in[0, 1]
\end{equation}
but not the other way around. 
\end{proposition}
The proof for Proposition  \ref{pro:2} can be found in \textbf{Need Appendix}. 


Based on Proposition \ref{pro:1} and \ref{pro:2}, we notice that Proportionality for Necessity and Sufficiency actually form a subset of the concept of \textit{sensitivity-n}. To approach the Proportionality in the other way, we show that:

\begin{proposition}
If an attribution method $A$ satisfy sensitivity-$n$ for all integer $n$ in [1, N], where N is the total number of pixels, then $N_p(X, A) = S_p(X, A) = 0$, but not the other way around. \label{pro:3}
\end{proposition}
\begin{proof}
\textit{If an attribution method A satisfies \textit{sensitivity-n} for all n in the range of $[1, N]$, where $N$ is the total number of pixels and given  $\forall n_1, n_2 \in [1, N]$, it satisfies \textit{sensitivity-$n_1$} and \textit{sensitivity-$n_2$} by definition. Based on Proposition \ref{pro:1}, 
$$N^k_p(X, A) = 0 \quad\text{for all possible k}$$Similarly, let $n_1 = N-n'_1, n_2 = N-n'_2$, so it satisfies \textit{sensitivity-$(N-n'_1)$} and \textit{sensitivity-$(N-n'_2)$}. Based on Proposition \ref{pro:2}, we have $$S^k_p(X, A) = 0 \quad \text{for all possible k}$$ Therefore, 
\begin{equation}
    N_p(X, A) = \int^1_0 N^k_p(X, A) dk = \int^1_0 0 dk = 0
\end{equation}
\begin{equation}
    S_p(X, A) = \int^1_0 S^k_p(X, A) dk = \int^1_0 0 dk = 0
\end{equation}}
\end{proof}
